# Supplementary material for: Versatility of type-II van der Waals heterostructures: a case study with SiH-CdCl2
Source: arXiv:2306.02048 ancillary file (2023-06-03)
Supplement: Supplementary file 1 [file SM_clean_01.pdf]

# Supporting Information for
# Versatility of type-II van der Waals heterostructures: a case study with SiH-$CdCl_2$

Achintya Priydarshi,[1,*] Abhinav Arora,[2] Yogesh Singh Chauhan,[1,†] Amit Agarwal,[3,‡] and Somnath Bhowmick[2,§]

[1]*Department of Electrical Engineering, Indian Institute of Technology Kanpur, Kanpur 208016, India*

[2]*Department of Materials Science and Engineering, Indian Institute of Technology Kanpur, Kanpur 208016, India*

[3]*Department of Physics, Indian Institute of Technology Kanpur, Kanpur 208016, India*

(Dated: May 14, 2023)

* achintya@iitk.ac.in

† chauhan@iitk.ac.in

‡ amitag@iitk.ac.in

§ bsomnath@iitk.ac.in

## I. LIST OF TABLES

**TABLE S1:** Structural parameters of relaxed isolated monolayers and their most stable heterostructure.

| Material | a = b (Å) | d (Å) | $L_{Cd-Cl}$ (Å) | $L_{Si-Si}$ (Å) | $L_{Si-H}$ (Å) |
|---|---|---|---|---|---|
| SiH | 3.86 | NA | NA | 2.34040 | 1.49749 |
| $CdCl_2$ | 3.80 | NA | 2.64740 | NA | NA |
| SiH/$CdCl_2$ | 3.84 | 2.14 | 2.65538 | 2.33436 | 1.49888 |

## II. LIST OF FIGURES

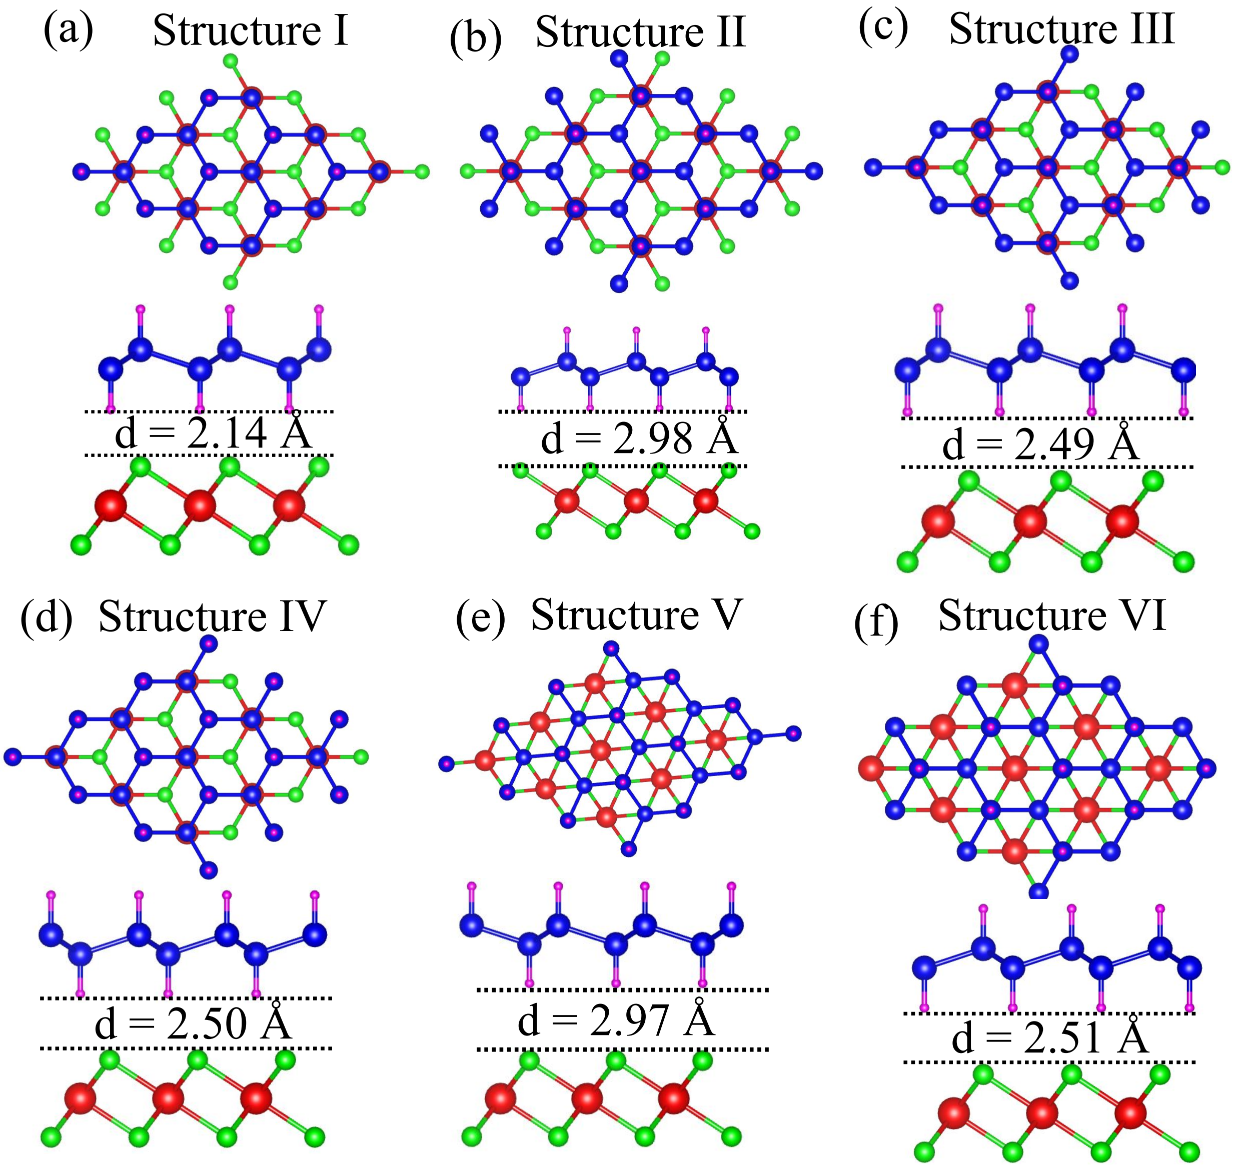


**FIG. S1:** (a)-(f) The top view and side view of all possible six heterostructure. We took structure-I for all of our calculations as it is the most stable among all.

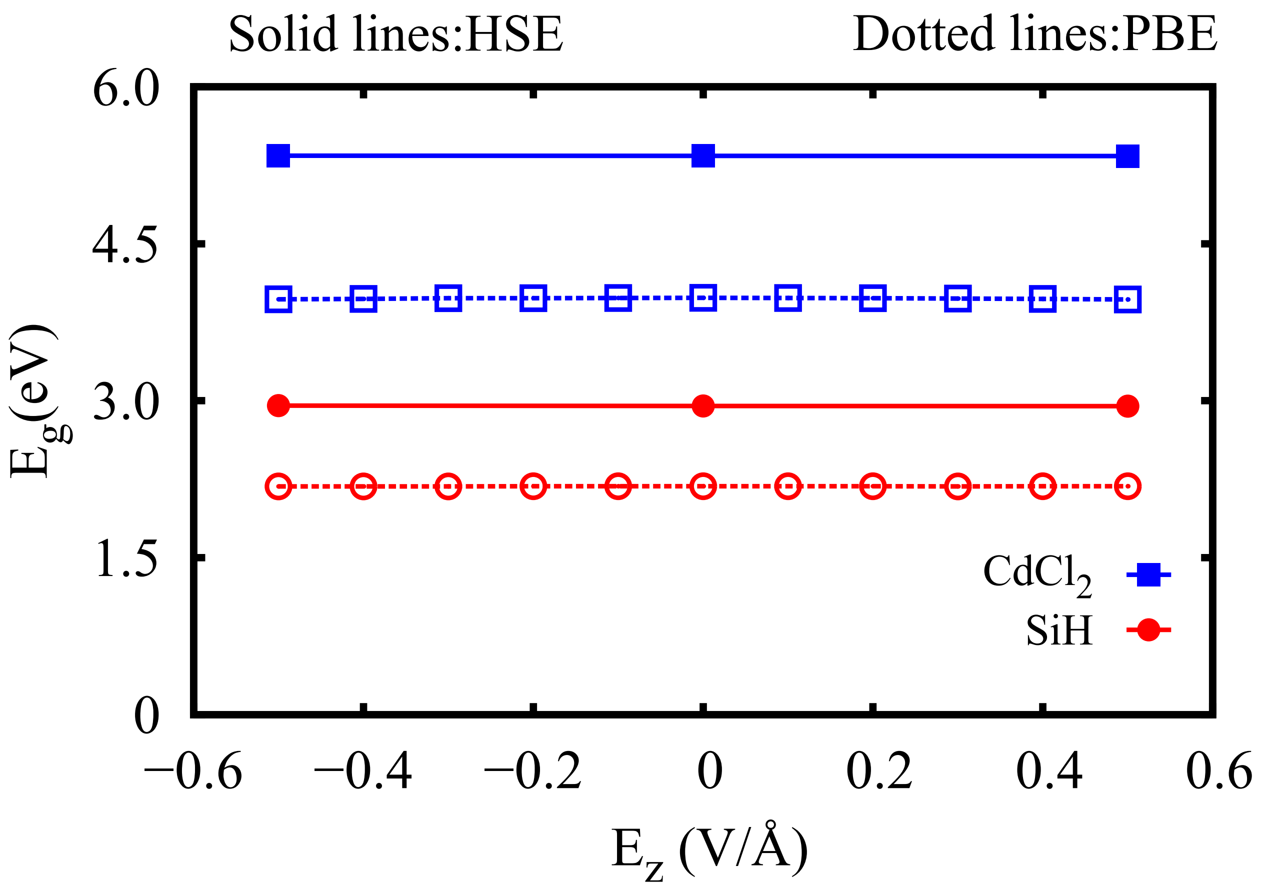


**FIG. S2:** The modification in the band gap of SiH and $CdCl_2$ monolayers as a function of vertical electric field $E_z$.

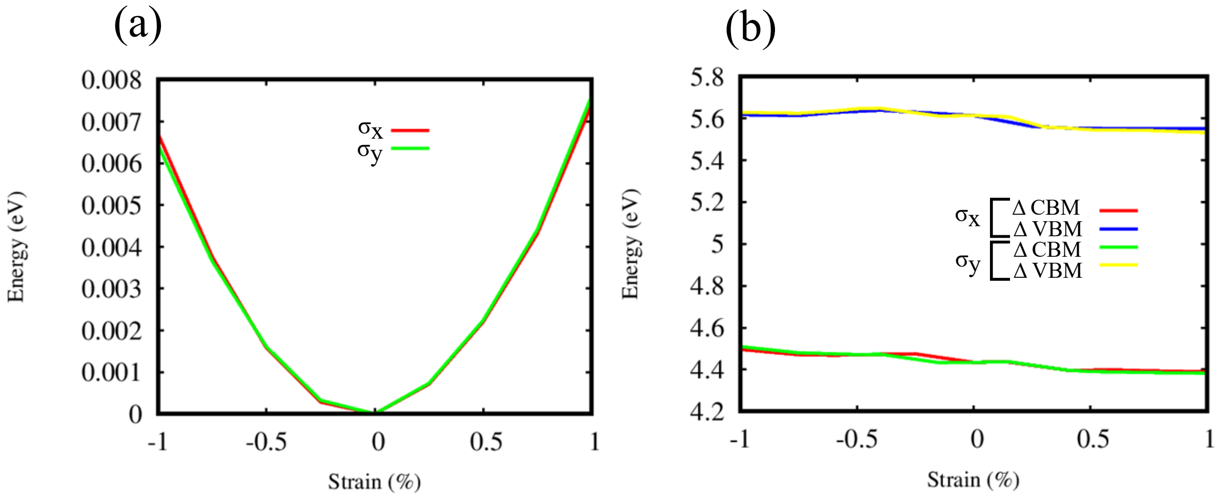


**FIG. S3:** (a) Energy-strain relationship in SiH/$CdCl_2$ heterostructre obtained by applying uniaxial strain along the $x$ and $y$ directions. (b) The uniaxial strain induced shift of the conduction and valence band edges for strain applied along the $x$ and $y$ directions.

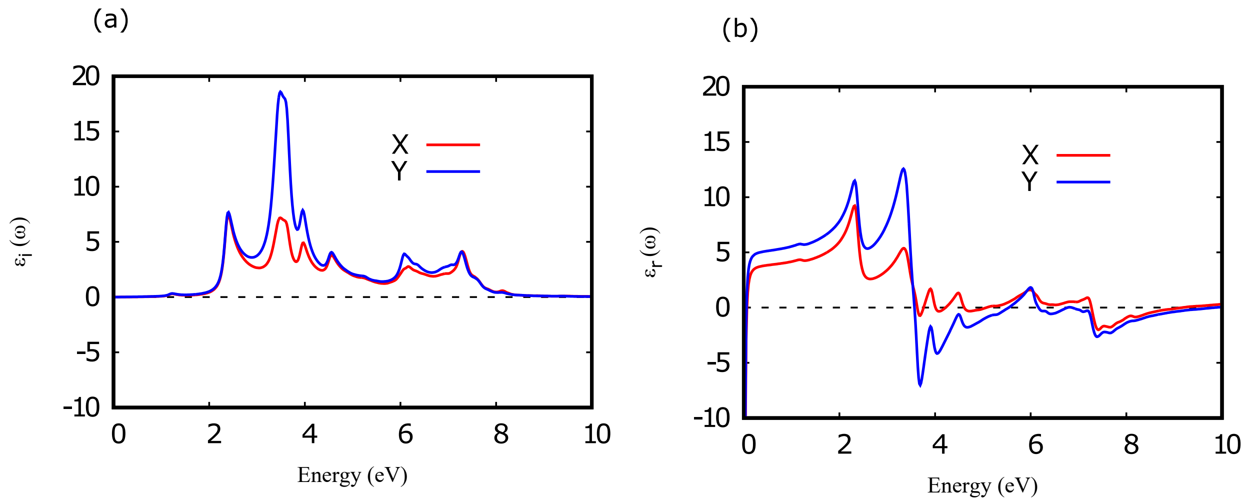


**FIG. S4:** Imaginary and real part of the dielectric functions in SiH/$CdCl_2$ heterostructre.

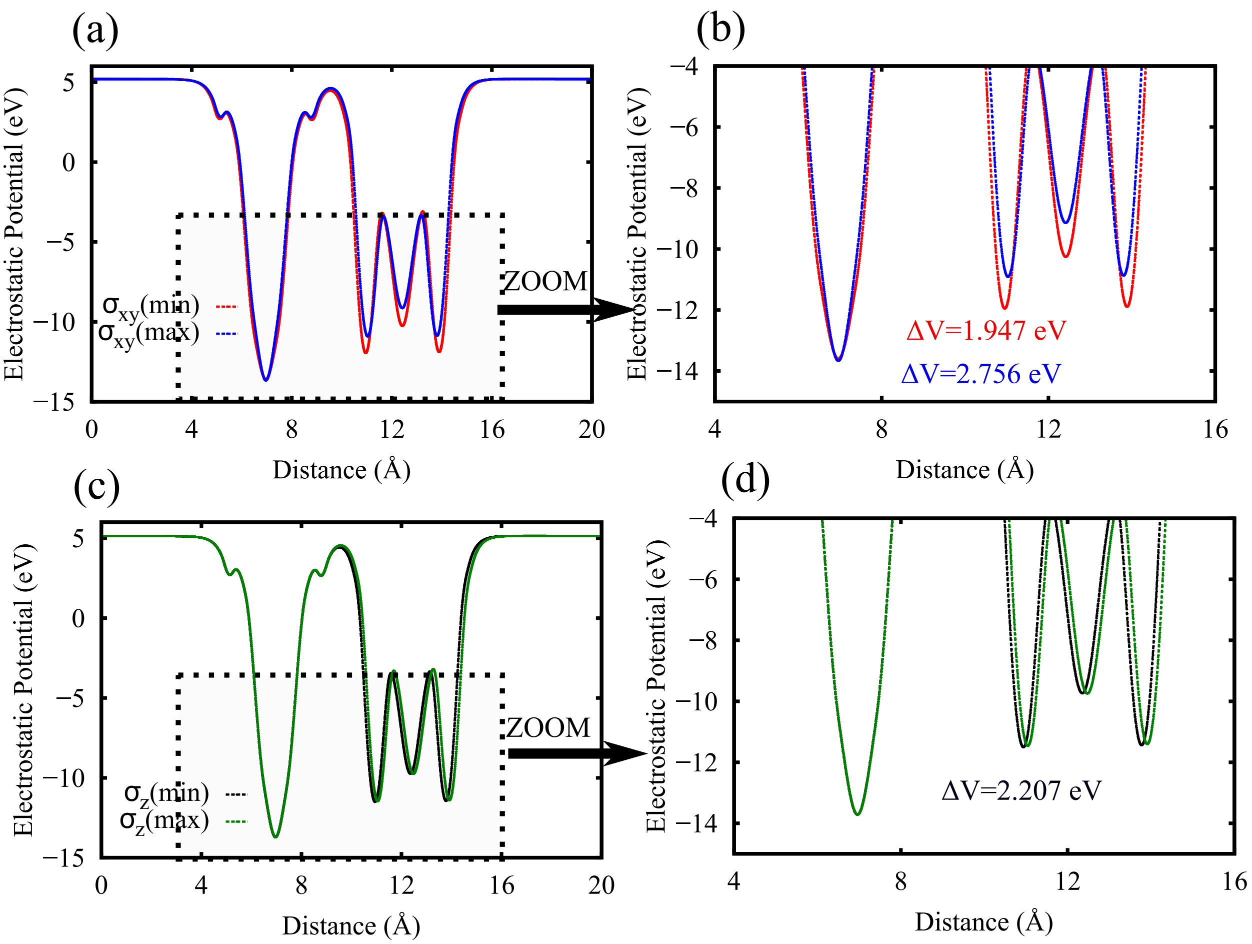


**FIG. S5:** Plane averaged potential along the height of the SiH/$CdCl_2$ heterostructure as a function of biaxial strain (a)-(b)and vertical strain (c)-(d).

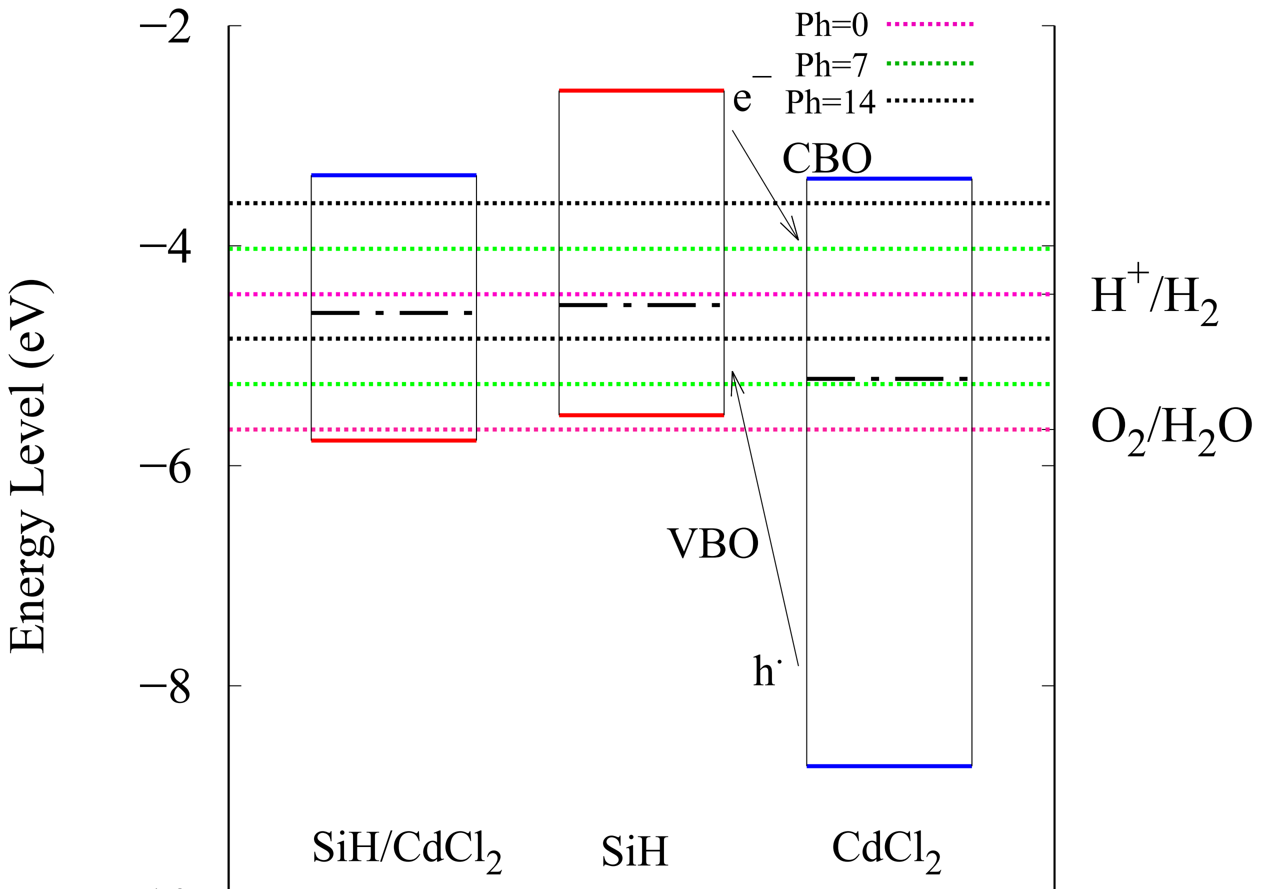


**FIG. S6:** Band diagram of isolated monolayers of SiH, $CdCl_2$ and their heterostructure at various pH values.

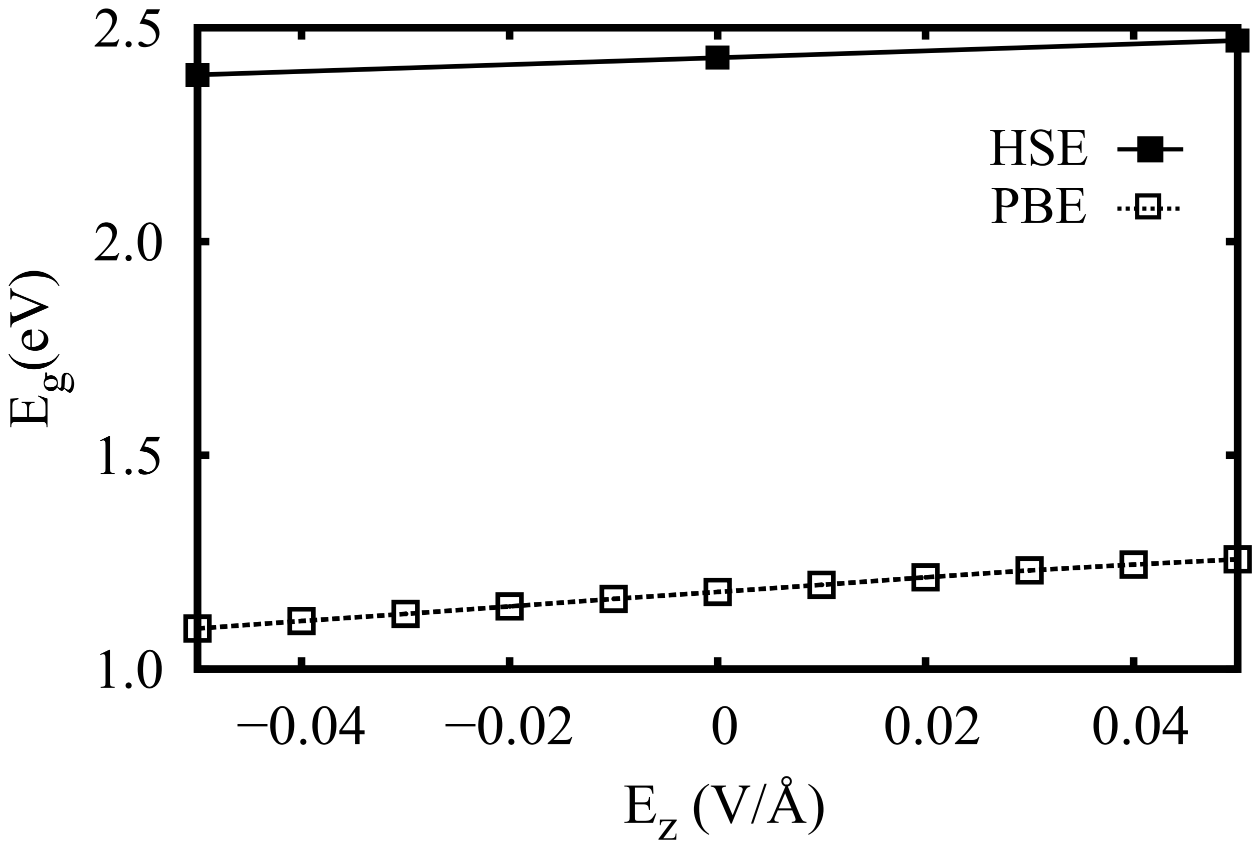


**FIG. S7:** The modification in the band gap of SiH/$CdCl_2$ heterostructure as a function of vertical electric field $E_z$.

## III. LIST OF EQUATIONS

The relationship between the redox potential of water and pH is shown below

$$E^{red} = -4.44\ eV + pH \times 0.059 \tag{S1}$$

$$E^{oxd} = -5.67\ eV + pH \times 0.059 \tag{S2}$$

where $E^{red}$ and $E^{oxd}$ represent the reduction and oxidation potential of water.
